# Supplementary material for: DoRA: Domain-Based Self-Supervised Learning Framework for Low-Resource Real Estate Appraisal
Source: arXiv:2309.00855 source file (2023-09-14)
Supplement: Supplementary file 1 [file 8-Appendix.tex]

\appendix
\section{Appendix}
\subsection{Details of the Features}
\label{feature-details}
Tables \ref{tab:data_details}, \ref{tab:data_details_2}, and \ref{tab:data-details-3} describe the details of each feature including feature types and examples of real estate features, PoI features, and economic and geographical features, respectively.

\begin{table*}
    \small
    \caption{Details of the real estate features in the dataset.}
    \label{tab:data_details}
    \begin{tabular}{c|cc}
    \toprule
    Feature & Feature Type (\#class) & Example \\
    \midrule
    City Name & Category (21) & Taipei city\\
    Town Name & Category (350) & Ren'ai township \\
    Parking spot & Category (2) & True/False (If the house includes a parking spot.) \\
    Studio & Binary & True/False (If the area of the estate is smaller than 8 square meters.) \\
    Details building type & Category (5) & Residential building (11 floors and above), Mansion (10 floors and below) \\
    Main Purpose & Category (1622) & Electromechanical equipment space \\
    Building materials & Category (220) & Rebar, Wood \\
    Management organization & Binary & True/False \\
    Type of parking space & Category (3) & Flat parking spot, Automated parking spot \\
    Elevator & Binary & True/False \\
    First-floor index & Binary &  True/False (If the house is located on the first floor.)\\
    Shop index & Binary &  True/False (If the house is for shop use.)\\
    Housing type & Category (3) & Building, Apartment, House \\
     % col2\_ind & Category(2) &  \\
    Village name & Category (4650) & Zhongshan village \\
    Land use & Category (19) & Residential zone, Forestry land, Mining land \\
    Land Use Designation & Category (16) & Type A building land, Class B building site \\
    Land transfer area & Numerical & 30 \\
    Building transfer area & Numerical & 50 \\
    Number of bedrooms & Numerical & 2 \\
    Number of living rooms & Numerical & 1 \\
    Number of bathroom & Numerical & 3 \\
    Number of total rooms & Numerical & 5 \\
    Parking area & Numerical & 5 \\
    Main building area & Numerical & 100 \\
    Ancillary building area & Numerical  & 10 \\
    Balcony area & Numerical & 5 \\
    House age & Numerical & 10 years \\
    Number of land transaction & Numerical & 1 \\
    Number of building transaction & Numerical &  1 \\
    Number of parking space transactions & Numerical & 2 \\
    Building area without parking area & Numerical & 45 \\
    Single floor area & Numerical & 20 \\
    Floor area ratio (FAR) & Numerical & 10 (Derived by dividing the total area of the building by the total area of the parcel.) \\
    Estate floor & Numerical & 5 \\
    Total floor & Numerical & 10 \\
    Latitude & Numerical & Horizontal lines that measure distance north or south of the equator \\
    Longitude & Numerical & Vertical lines that measure east or west of the meridian in Greenwich, England. \\
    Building coverage ratio & Numerical & 9 \\
    Park count flat & Numerical &  0 \\
    \bottomrule
\end{tabular}
\end{table*}

\begin{table*}
    \caption{Details of the PoI features in the dataset.}
    \label{tab:data_details_2}
    \begin{tabular}{c|cc}
    \toprule
   Feature & Feature Type (\#class) & Example \\
    \midrule
    YIMBY\_10 & Numerical & 2\\
    YIMBY\_50 & Numerical & 3\\
    YIMBY\_100 & Numerical & 3\\
    YIMBY\_250 & Numerical & 6\\
    YIMBY\_500 & Numerical & 7\\
    YIMBY\_1000 & Numerical & 13\\
    YIMBY\_5000 & Numerical & 28\\
    YIMBY\_10000 & Numerical & 52\\
    \midrule
    NIMBY\_10 & Numerical &  0\\
    NIMBY\_50 & Numerical &  0\\
    NIMBY\_100 & Numerical &  0\\
    NIMBY\_250 & Numerical &  1\\
    NIMBY\_500 & Numerical &  1\\
    NIMBY\_1000 & Numerical &  2\\
    NIMBY\_5000 & Numerical &  3\\
    NIMBY\_10000 & Numerical &  6\\
    \bottomrule
\end{tabular}
\end{table*}

\begin{table*}
    \caption{Details of the economic and geographical features in the dataset.}
    \label{tab:data-details-3}
    \begin{tabular}{c|cc}
    \toprule
    Feature & Feature Type (\#class) & Example \\
    \midrule
    Land area per town & Numerical & 23.13 (km\textsuperscript{2}) \\
    Population density per town & Numerical & 23835 (\#people/km\textsuperscript{2}) \\
    House price index per quarter & Numerical & 110 \\
    Unemployment rate per quarter & Numerical & 5\% \\
    Economic growth rate per quarter & Numerical & 3\% \\
    Lending rate per quarter & Numerical & 1.9\% \\
    Land transaction count per quarter & Numerical & 163796 \\
    Average land price index per quarter & Numerical & 101 \\
    Steel price index per quarter & Numerical & 1071 \\
    \bottomrule
\end{tabular}
\end{table*}

\subsection{Code and Data}
\label{code-and-data}
% \subsubsection{Code and Data}
Since there is no official place for reducibility, we provide our code and sample data in the link\footnote{shorturl.at/aeIMV}.
We release only part of the datasets due to the license restriction.

% \subsubsection{HR20\% and RMSE Performance}
% \label{mae_rmse_performance}
% Table \ref{tab:1shot_2} and Table \ref{tab:5shot_2} show the performance evaluated by HR20\% and RMSE of all baselines and DoRA with 1 and 5 shots scenarios, which illustrates that DoRA still consistently surpasses other baselines.
% Also, similar conclusions can be observed by using MAPE, HR10\%, and MAE metrics.

\subsection{Other Metrics of Model Ablation}
Table \ref{tab:ablation_2} presents other metrics for studying model ablation.
We can reach the same conclusions by using the MAPE metric.

% \begin{table*}
%     \centering
%     \caption{Overall 1 shot performance evaluated by HR20\% and RMSE on the Building, Apartment, and House datasets.}
%     \label{tab:1shot_2}
%     \input{Table/1shot_2.tex}
% \end{table*}

% \begin{table*}
%     \centering
%     \caption{Overall 5 shots performance evaluated by HR20\% and RMSE on the building, apartment, and house datasets.}
%     \label{tab:5shot_2}
%     \input{Table/5shot_2.tex}
% \end{table*}

\begin{table*}
    \caption{Ablation study with HR10\% and MAE using the building dataset in the 5-shot setting. }
    \label{tab:ablation_2}
    \newcommand{\specialcell}[2][c]{%
  \begin{tabular}[#1]{@{}c@{}}#2\end{tabular}}

\begin{tabular}{ccccc|cc}
    \toprule
    \specialcell{Pre-Trained\\Datasets} & \specialcell{Pretext\\Task} & CL ($\alpha$) & $d_Z$ & \specialcell{Fine-Tune\\Encoder} & MAE ($\downarrow$) & HR10\% ($\uparrow$) \\
    \midrule
    \midrule
    Building & Town & + (0.7) & 256 & \cmark & 12.05 & 15.25 \\
    \midrule
    All & Town & + (0.7)  & 512 & \cmark & 9.22 & 19.24 \\
    \midrule
    All & Town & + (0.7) & 256 & \xmark & 15.16 & 7.41 \\
    \midrule
    All & Town & - & 256 & \cmark & 11.51 & 13.48 \\
    \midrule
    All & Town & + (0.5) & 256 & \cmark & 12.79 & 14.99 \\
    \midrule
    \midrule
    All & City & + (0.7) & 256 & \cmark & 10.88 & 17.8 \\
    \midrule
    All & Parking Spot & + (0.7) & 256 & \cmark & 11.61 & 14.63 \\
    \midrule
    All & House Age & + (0.7) & 256 & \cmark & 9.64 & 18.43 \\
    \midrule
    All & Floor & + (0.7) & 256 & \cmark & 9.64 & 18.05 \\
    \midrule
    \midrule
    All & Town & + (0.7) & 256 & \cmark & \textbf{7.79} & \textbf{20.16} \\
    \bottomrule
\end{tabular}

% \begin{tabular}{ccccc|ccc}
%     \toprule
%     \specialcell{Pre-Trained\\Datasets} & \specialcell{Pretext\\Task} & CL ($\alpha$) & $d_Z$ & \specialcell{Fine-Tune\\Encoder} & MAPE ($\downarrow$) & MAE ($\downarrow$) & HR10\% ($\uparrow$) \\
%     \midrule
%     \midrule
%     Building & Town & + (0.7) & 256 & \cmark & 37.09 & 12.05 & 15.25 \\
%     \midrule
%     All & Town & + (0.7)  & 512 & \cmark & 33.65 & 9.22 & 19.24 \\
%     \midrule
%     All & Town & + (0.7) & 256 & \xmark & 58.65 & 15.16 & 7.41 \\
%     \midrule
%     All & Town & - & 256 & \cmark & 37.83 & 11.51 & 13.48 \\
%     \midrule
%     All & Town & + (0.5) & 256 & \cmark & 36.37 & 12.79 & 14.99 \\
%     \midrule
%     \midrule
%     All & City & + (0.7) & 256 & \cmark & 36.38 & 10.88 & 17.8 \\
%     \midrule
%     All & Parking Spot & + (0.7) & 256 & \cmark & 38.13 & 11.61 & 14.63 \\
%     \midrule
%     All & House Age & + (0.7) & 256 & \cmark & 32.37 & 9.64 & 18.43 \\
%     \midrule
%     All & Floor & + (0.7) & 256 & \cmark & 34.9 & 9.64 & 18.05 \\
%     \midrule
%     \midrule
%     All & Town & + (0.7) & 256 & \cmark & \textbf{31.85} & \textbf{7.79} & \textbf{20.16} \\
%     \bottomrule
% \end{tabular}
\end{table*}

% \begin{table}
%     \small
%     \caption{Case study: Analysis of the top 5 least data city in the building dataset with 5 shots setting. }
%     \input{Table/case_study.tex}
%     \label{tab:case-study}
% \end{table}

% \subsection{Case Study: Few-shot Scenario - Take the Top 5 Smallest City as Example}
% \label{case_study}
% To demonstrate the low resource scenario, we group by the city name and then calculate each city's testing performance.
% Table \ref{tab:case-study} shows the top 5 less building city MAPE.
% In most cases, DoRA outperforms XGBoost, which proves that DoRA is more outstanding in few-shot settings.
